# Supplementary material for: The liquid state of one-dimensional Bose mixtures: a quantum Monte-Carlo study
Source: arXiv:1810.07950 source file (2018-10-18)
Supplement: Supplementary file 1 [file 1DdropletsSupplemental.pdf]

# The liquid state of one-dimensional Bose mixtures: a quantum Monte-Carlo study: Supplemental Material

L. Parisi[1], G. E. Astrakharchik[2] and S. Giorgini[1]

[1] *Dipartimento di Fisica, Università di Trento and CNR-INO BEC Center, I-38050 Povo, Trento, Italy*

[2] *Departament de Física i Enginyeria Nuclear, Universitat Politècnica de Catalunya, Campus Nord B4-B5, E-08034, Barcelona, Spain*

## I. CHOICE OF THE GUIDING WAVE FUNCTION

The guiding wave function of the positions $x_i$ and $x_\alpha$ of particles respectively from the component $a$ and $b$ is chosen as

$$\psi_T(x_1,\ldots,x_{N_a};x_1,\ldots,x_{N_b}) = \prod_{i<j} f(x_i - x_j) \prod_{\alpha<\beta} f(x_\alpha - x_\beta) \prod_{i,\alpha} h(x_i - x_\alpha) \;, \tag{1}$$

where $f(x)$ and $h(x)$ are pair-wise Jastrow terms corresponding, respectively, to intra-species and inter-species correlations. Contact interactions are simulated by requiring that $f(x)$ and $h(x)$ satisfy the proper boundary conditions at the origin[1]. In particular, we choose $f(x) = \sin(k|x| + \varphi(k))$ if $|x| < X_m$ and $f(x) = \sin^\beta(\pi|x|/L)$ if $X_m < |x| < L/2$. The parameters $k$ and *beta* are fixed by the continuity condition of the function $f(x)$ and its first derivative at the matching point $X_m$. For $|x| > X_m$ the Jastrow function takes into account long-range correlations due to phonon excitations[2]. The phase shift results from the contact condition imposed by the interatomic potential and is given by $\varphi(k) = \arctan\frac{2\hbar^2 k}{mg}$. The function $h$ is chosen as $h(x) = (e^{-k(|x|-L/2)} + e^{k(|x|-L/2)})/2$ for $|x| < L/2$. The parameter $k$ is fixed by the condition: $kL/2 = \tanh^{-1}(1/k\tilde{a})$ in terms of the inter-species scattering length $\tilde{a}$. We notice that both $f'(x) = 0$ and $h'(x) = 0$ at $|x| = L/2$ in compliance with the periodic boundary conditions of the system. The matching point $X_m$ is a variational parameter optimized by minimizing the expectation value $\langle\psi_T|H|\psi_T\rangle$ of the Hamiltonian on the many-body state $\psi_T$.

[1] L. Parisi and S. Giorgini, Phys. Rev. A **95**, 023619 (2017).

[2] L. Reatto and G. V. Chester, Phys. Rev. **155**, 155 (1967).
